# Supplementary material for: Instance Segmentation as Image Segmentation Annotation
Source: arXiv:1902.05498 source file (2019-02-01)
Supplement: Supplementary file 1 [file appendix.tex]

\section*{Appendix}

\begin{figure*}[ht]
\begin{center}
	  \begin{subfigure}{\textwidth}
        \includegraphics[scale=.65]{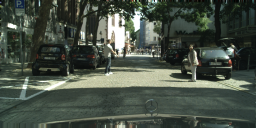}
        \vspace{1mm}
        \includegraphics[scale=.65]{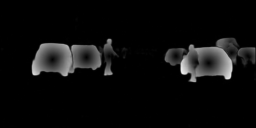}
        \includegraphics[scale=.65]{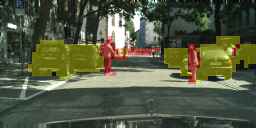}
    \end{subfigure}
    \vspace{1mm}
    \begin{subfigure}{\textwidth}
        \includegraphics[scale=.65]{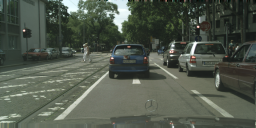}
        \includegraphics[scale=.65]{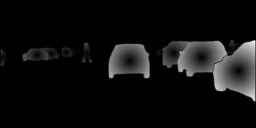}
        \includegraphics[scale=.65]{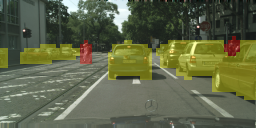}
    \end{subfigure}
    \vspace{1mm}
    \begin{subfigure}{\textwidth}
        \includegraphics[scale=.65]{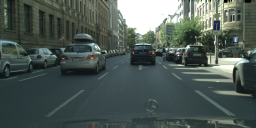}
        \includegraphics[scale=.65]{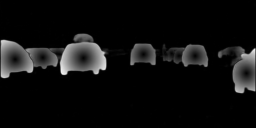}
        \includegraphics[scale=.65]{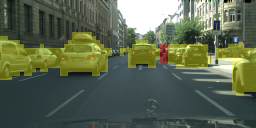}
    \end{subfigure}
    \vspace{1mm}
    \begin{subfigure}{\textwidth}
        \includegraphics[scale=.65]{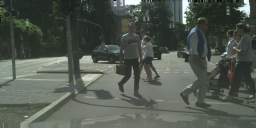}
        \includegraphics[scale=.65]{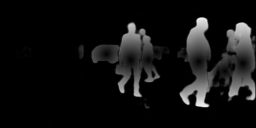}
        \includegraphics[scale=.65]{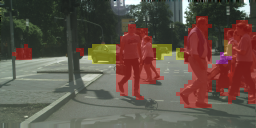}
    \end{subfigure}
    \vspace{1mm}
    \begin{subfigure}{\textwidth}
        \includegraphics[scale=.65]{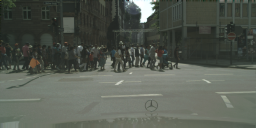}
        \includegraphics[scale=.65]{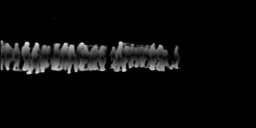}
        \includegraphics[scale=.65]{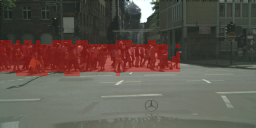}
    \end{subfigure}
    \vspace{1mm}
\end{center}
\caption{From left to right: input images, 2D vectors magnitude map and class map.}
\label{fig:deeplab_v4}
\end{figure*}
